# Supplementary material for: A spectral-neighbour representation for vector fields: machine-learning potentials including spin
Source: arXiv:2202.13773 source file (2022-08-08)
Supplement: Supplementary file 1 [file MB4VectorField_SI.pdf]

# Supplementary Informations
# A spectral-neighbour representation for vector fields: machine-learning potentials including spin

M. Domina, M. Cobelli, and S. Sanvito

*School of Physics and CRANN Institute, Trinity College Dublin, Ireland*

The Table below reports the details of the fittings performed. It is divided in the two section, namely "Ferromagnetic" and "Random" training sets, referring to the datasets introduced in the main text. The training parameters are the maximum degree of the expansion, the cut-off radius, and the regolarization constant for the linear regression. The MAEs reported are that obtained from the fit on the Train and on the Test sets, described in detail in the main text. The Prediction's MAE refers to the MAE predicted on the dataset spanning the full energy range, which is detailed in the parity plots below, one for each training set. The Upper's MAEs report the results for energies > 0.01 eV/atom present in the "Prediction" set. This region is highlighted in the inserts of the plots below. For the case of the "Ferromagnetic" training sets it is an estimation of the extrapolation power of the model. On the contrary, for the "Random" training sets, which spans a smaller range of the energies, it is an estimation of the interpolation. The learning curves are reported as a sanity check against overfitting.

"Ferromagnetic" training sets

| | Training Parameters | | | MAEs (eV/atom) | | | |
|---|---|---|---|---|---|---|---|
| Max Displacement | $n_{\max}$ | $r_{\text{cut}}$ (lattice units) | $\alpha$ | Train | Test | Prediction | Upper |
| 5% | 5 | 1.4 | $1.7 \times 10^2$ | $(1.03 \pm 0.07) \times 10^{-5}$ | $(2.05 \pm 0.14) \times 10^{-5}$ | $7.3 \times 10^{-5}$ | $6.9 \times 10^{-5}$ |
| 10% | 4 | 1.4 | $3.2 \times 10^3$ | $(4.83 \pm 0.15) \times 10^{-5}$ | $(6.8 \pm 0.7) \times 10^{-5}$ | $5.6 \times 10^{-4}$ | $8.2 \times 10^{-4}$ |
| 20% | 6 | 1.35 | $3.9 \times 10^4$ | $(1.39 \pm 0.12) \times 10^{-4}$ | $(2.7 \pm 0.3) \times 10^{-4}$ | $6.1 \times 10^{-4}$ | $1.1 \times 10^{-3}$ |

"Random" training sets

| | Training Parameters | | | MAEs (eV/atom) | | | |
|---|---|---|---|---|---|---|---|
| Max Displacement | $n_{\max}$ | $r_{\text{cut}}$ (lattice units) | $\alpha$ | Train | Test | Prediction | Upper |
| 5% | 5 | 1.45 | $1.9 \times 10^2$ | $(1.74 \pm 0.04) \times 10^{-5}$ | $(4.7 \pm 0.3) \times 10^{-5}$ | $1.3 \times 10^{-4}$ | $4.9 \times 10^{-5}$ |
| 10% | 4 | 1.4 | $8.4 \times 10^2$ | $(6.5 \pm 0.3) \times 10^{-5}$ | $(1.23 \pm 0.09) \times 10^{-4}$ | $2.5 \times 10^{-3}$ | $8.3 \times 10^{-4}$ |
| 20% | 4 | 1.4 | $2.1 \times 10^4$ | $(2.30 \pm 0.09) \times 10^{-4}$ | $(3.8 \pm 0.3) \times 10^{-4}$ | 0.01 | $3.20 \times 10^{-3}$ |

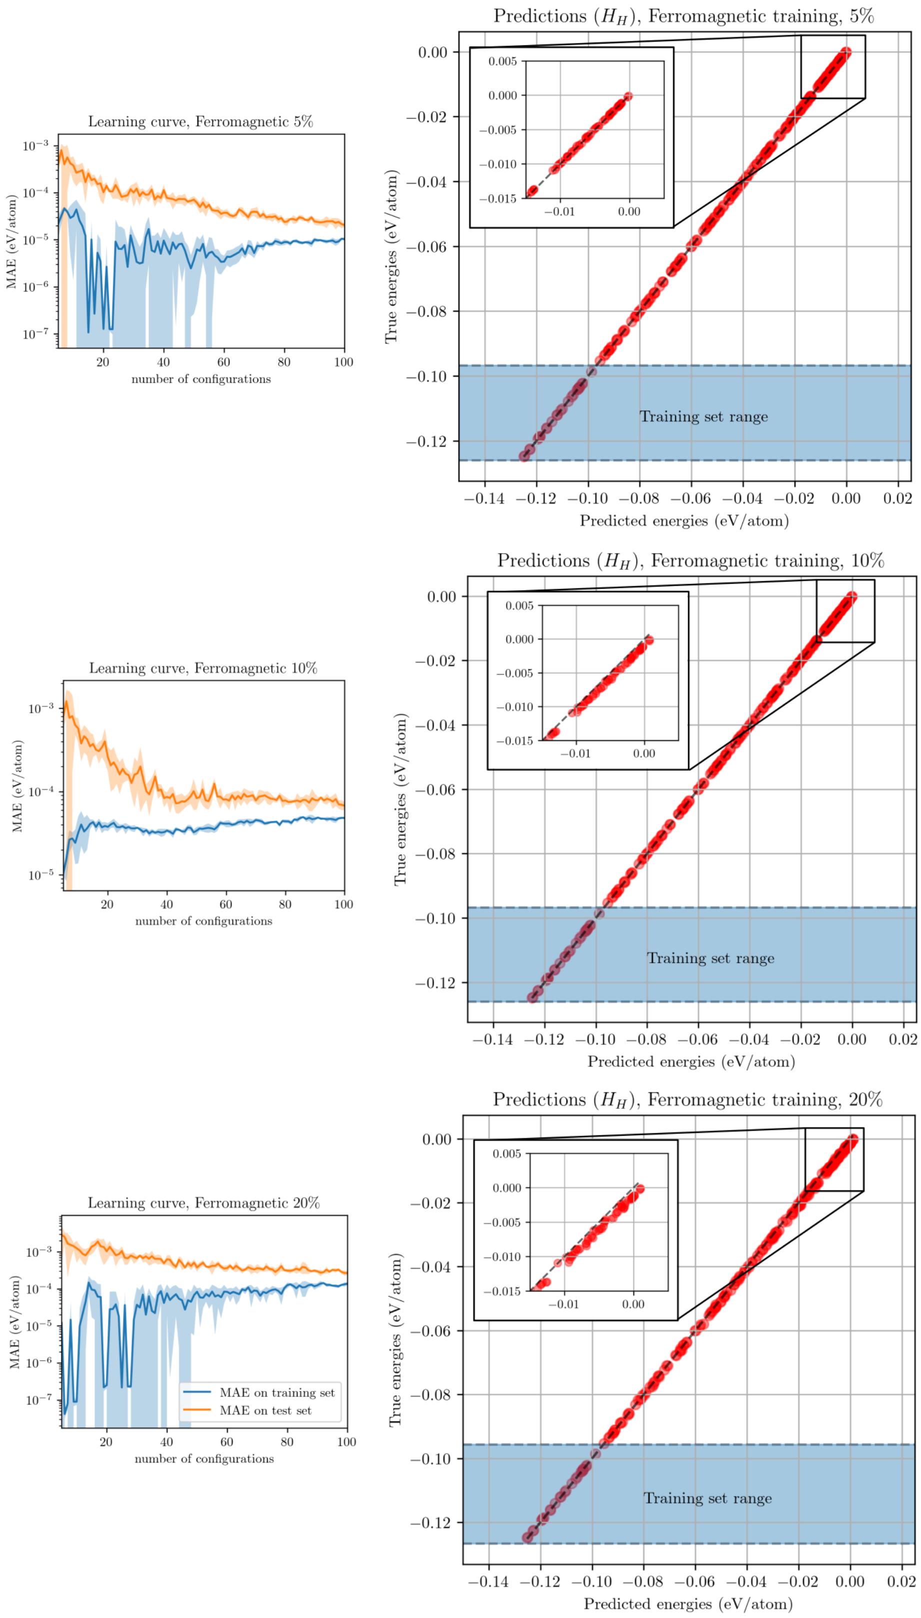


FIG. 1. Learning curves and predictions of the models trained on the "Ferromagnetic" training sets, with zoom-in in the extrapolation region. The percentages in the titles label the maximum displacement of the training set. More details are present in the main text.

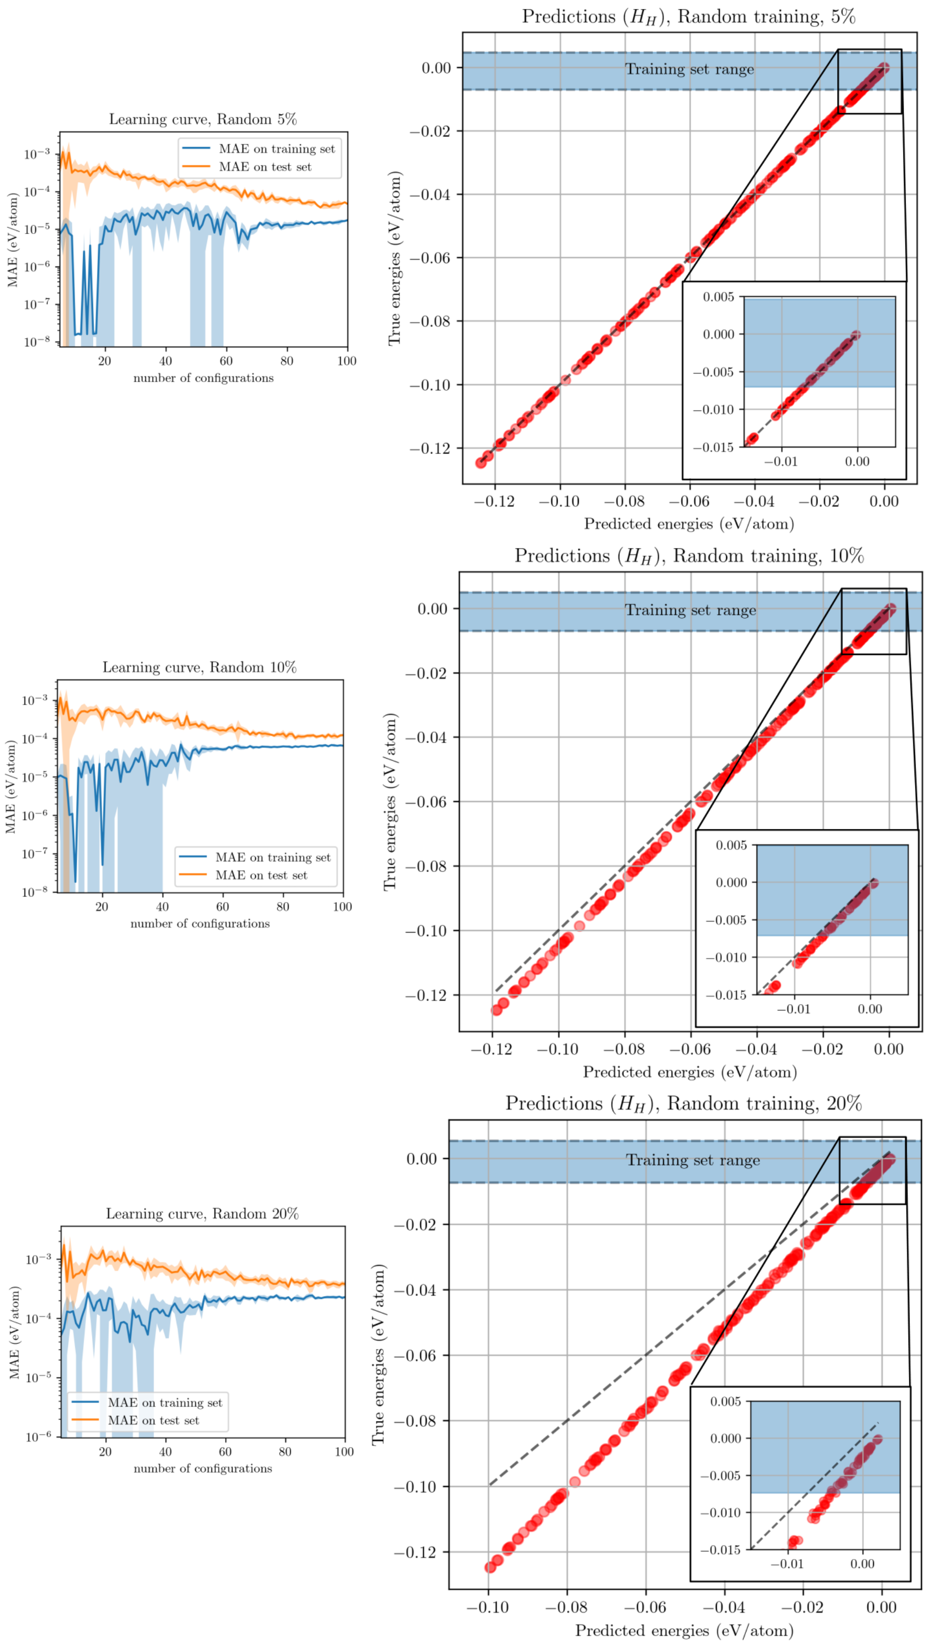


FIG. 2. Same plots for the models trained on the "Random" training sets, with zoom-in in the interpolation region.
